# Supplementary material for: SPINEPS -- Automatic Whole Spine Segmentation of T2-weighted MR images using a Two-Phase Approach to Multi-class Semantic and Instance Segmentation
Source: arXiv:2402.16368 source file (2024-04-22)
Supplement: Supplementary file 1 [file appendix.tex]

\clearpage
\setcounter{section}{41}
\section{Appendix}
\input{body/appendix/benchmark}
